# Supplementary material for: Maximum Likelihood Estimation for Brownian Motion Tree Models Based on One Sample
Source: arXiv:2112.00816 source file (2022-11-24)
Supplement: Supplementary file 1 [file old_appendix.tex]

\section{Tree metrics, Brownian tree models,  and Laplacians}

In this section we present a convenient coordinate change that links Brownian motion tree models to tree metrics and Laplacians on graphs. 

Let $\S^d$ denote the space of real symmetric $d\times d$ matrices and $\S^d_0$ its subspace given by matrices with zeros on the diagonal. The space $\S^d$ is equipped with the usual trace inner product $\<A,B\>=\tr(AB)$ and the inner product on $\S^d_0$ is
$$
\langle\!\langle A,B\rangle\!\rangle\;=\;\frac12\tr(AB)\;=\;\sum_{0\leq i<j\leq d} A_{ij}B_{ij}.
$$
We write $\bs 1$ for the vector of ones, $\bs 0$ for the vector of zeros, and $I_d$ for the identity matrix.

Consider $\S^{d+1}$ with row/columns indexed by $0,\ldots,d$. Denote $\mathbb V=\S^{d+1}_0$. Let $\mathbb U$ and $\mathbb U_0$ be two subspaces of $\S^{d+1}$ given by matrices $A\in \S^d$ that satisfy $A\bs 1=\bs 0$ ($A\bs e_0=\bs 0$ resp.), where $\bs e_0$ is the 0-th canonical unit vector in $\R^{d+1}$. We identify $\mathbb U_0$ with $\S^d$ in an obvious way: the elements of $\mathbb U_0$ are denoted with a bar above and the corresponding elements of $\S^d$ are denoted without the bar. For example, if $\overline A\in \mathbb U_0$, then $A\in \S^d$ is the matrix obtained from $\overline A$ by deleting the 0-th row and column. 

Let $\bs P_{ 0}=I_{d+1}-\bs 1 \bs e_0^T$ and $\bs P=I_{d+1}-\frac{1}{d+1}\bs 1\bs 1^T$ be two $(d+1)\times (d+1)$ matrices. In what follows we consider different copies of the spaces $\mathbb V, \mathbb U, \mathbb U_0$, which we distinguish by giving them different coordinate systems indicated in square brackets. Consider the following commuting diagram
\[\begin{tikzcd}
\mathbb V[D] \arrow[r,"\sigma_0"]  \arrow[dr,swap,"\sigma"] & \mathbb U_0 [\overline\Sigma] \arrow[r,"{\rm ginv}"]  & \mathbb U_0 [\overline K] \arrow[d,swap,"f^*"]  \arrow[r,"\sigma^*_0"] & \mathbb V [P]\\
  & \mathbb U[\Xi] \arrow[r,"{\rm ginv}"] \arrow[u,swap,"f"] & \mathbb U [L] \arrow[ru,swap,"\sigma^*"]& 
\end{tikzcd},
\]
where ${\rm ginv}$ denotes the generalized inverse $A\mapsto A^+$, and the three mappings on the left are linear and given by
$$
\sigma_{ 0}(D)\;=\;\bs P_{0} \left(-\tfrac{D}{2}\right)\bs P_0^T,\;\;\sigma(D)\;=\;\bs P \left(-\tfrac{D}{2}\right)\bs P,\;\;f(\Xi)=\bs P_{0} \Xi \bs P_0^T.
$$
The mappings $\sigma_0^*, \sigma^*,f^*$ are the adjoint mappings, that is, they are defined as the unique linear mappings that satisfy:
\begin{enumerate}
    \item $\< f(\Xi),\overline K\>=\<\Xi,f^*(\overline K)\>$ for all $\Xi,K$,
    \item $\<\sigma(D),L\>=\<\!\<D,\sigma^*(L)\>\!\>$ and $\<\sigma_0(D),\overline K\>=\<\!\<D,\sigma^*_0(\overline K)\>\!\>$ for all $D,L,\overline K$.
\end{enumerate}
By standard properties of the matrix trace we get that $f^*(\overline K)=\bs P_0^T L \bs P_0$. To find the formula for $\sigma^*$ we use the fact that
$$
\<\sigma(D),L\rangle=\frac12\<D,-\bs P L\bs P\>=\frac12\<D,- L\>=\sum_{0\leq i<j\leq d} D_{ij}(-L_{ij}),
$$
where the first equality follows by definition and basic properties of the trace and the second equality follows because $L\in \mathbb U$ implies that $\bs P L\bs P=L$. For the right hand side $\tfrac12\<D,- L\>$ to be equal to $\<\!\<C,\sigma^*(L)\>\!\>$ we need
$$
(\sigma^*(L))_{ij}=-L_{ij} \quad\mbox{for all }0\leq i<j\leq d.
$$
The fact that the diagram above commutes essentially follows from the fact that $\bs P_0\bs P=\bs P_0$, $\bs P^+=\bs P$, and $\bs P^+_0=\bs P(I_{d+1}-\bs e_0\bs e_0^T)$.

Let $T$ be a rooted tree with $n$ nodes and $d+1$ labeled nodes (the root labeled with $0$). Let $\theta_i$ denote the length of the edge connecting the node $i$ and its parent $\pi(i)$. The induced tree metric $D\in \mathbb V$ is given by $D_{ij}=\sum_{dd}dd$. We denote by $\mathbb D_T$ the set of all tree metrics over $T$ (all possible edge length assignments). 
\begin{prop}
The set $\mathbb D_T$ is mapped by $\sigma_0$ precisely to 
the Brownian motion tree model over $T$. It image in $\mathbb V[P]$ satisfies $P_{ij}\geq 0$ for all $i<j$.
\end{prop}
\begin{proof}
By definition $\Sigma=\sigma_{0}(D)$ is given by 
$\Sigma_{ij}=\frac{1}{2}\left(D_{0i}+D_{0j}-D_{ij}\right)$. If $D\in \mathbb D_T$ then $\Sigma_{ij}$ is precisely the sum of all $\theta_k$ for $k$ that lie on the path between $0$ and the most recent common ancestor of $i$ and $j$. This is precisely how BMTM is parameterized. 
\end{proof}

Let $\mathbb C\subset \mathbb U_0[K]$ be the cone of all matrices with $d$ strictly positive eigenvalues. Let $\mathbb D\subset \mathbb C$ be the subcone that is mapped to the nonnegative orthant by $\sigma^*_0$. (We should show that this image is simply the set of all nonnegative $P$ such that the underlying support is connected. )

We also note
$$
\log\det K-\tr(SK)\;=\;\log\sum_{S\in \mathcal T}\prod_{uv\in S}P_{uv}-\<\!\<D^S,P\>\!\>,
$$
where $D^S$ satisfies $\sigma_0(D^S)=\overline{S}$. This follows easily by...

We have also have a compact way of writing the inverse map from $P$ to $D$:
$$
D\;=\;\nabla_P \log\sum_{S\in \mathcal T}\prod_{uv\in S}P_{uv}.
$$
